# Supplementary material for: GUI-Xplore: Empowering Generalizable GUI Agents with One Exploration
Source: arXiv:2503.17709 source file (2025-03-22)
Supplement: Supplementary file 1 [file X_suppl.tex]

\clearpage
\setcounter{page}{1}
\maketitlesupplementary

\section{Rationale}
\label{sec:rationale}
\begin{table*}[htbp]
  \centering
  \begin{tabular}{@{}ccccccc@{}}
    \toprule
    View Hierarchy   & Action      & Overview       & Page          & Usage         & Recall        & SeqVeri \\ 
    \midrule
    \multicolumn{2}{c}{ScreenShot} & 96.88\%        & 82.12\%       & 66.48\%       & 19.60\%       & 22.53\%\\ 
    \midrule
    Generated        & -           &                &               &               &               &         \\
    GT               & -           &                &               &               &               &         \\
    Generated        & GT          & 99.25\%        & 97.25\%       & 68.35\%       & 24.20\%       & 29.72\%   \\
    GT               & Generated   & 99.62\%        & 96.34\%       & 67.79\%       & 23.70\%       & 25.88\% \\
    GT               & GT          & 99.63\%        & 92.86\%       & 67.40\%       & 24.54\%       & 26.71\% \\
    \midrule
    Generated        & Generated   & 99.25\%        & 92.86\%       & 68.21\%       & 24.36\%       & 36.54\%  \\
    \bottomrule
  \end{tabular}
  \caption{Comparison of different configurations across view hierarchy and action settings.}
  \label{tab:view_hierarchy_comparison}
\end{table*}
